# Supplementary material for: TFDNet: Time-Frequency Enhanced Decomposed Network for Long-term Time Series Forecasting
Source: arXiv:2308.13386 source file (2023-08-25)
Supplement: Supplementary file 1 [file univariate_datasets.tex]

\section{Univariate Forecasting}
\label{app:univariate}
